# Supplementary material for: Validation of 3GPP TR 38.901 Indoor Hotspot Path Loss Model Based on Measurements Conducted at 6.75, 16.95, 28, and 73 GHz for 6G and Beyond
Source: arXiv:2504.15589 source file (2025-04-22)
Supplement: Supplementary file 1 [file appendix.tex]

% \begin{table}[htbp]
%   \centering
%   \caption{Add caption}
%     \begin{tabular}{|c|p{1.6em}|p{1.6em}|p{1.8em}|p{2.4em}|p{1.9em}|p{2em}|}
% \hline
%     \multicolumn{7}{|c|}{6.75 GHz Omnidirectional V-V PL, DS and ASA} \\
% \hline
%     Env.  & TX ID & RX ID & T-R (m) & PL (dB) & DS (ns) & ASA ($^\circ$)\\
% \hline
%     LOS   & TX1   & RX1   & 24.6  & 68.2 &     21.4  & NA \\
% \hline
%     LOS   & TX1   & RX4   & 51    & 79.2 &     47.5  & 59.3 \\
% \hline
%     LOS   & TX2   & RX1   & 64    & 73 &     69.5  & 68.7 \\
% \hline
%     LOS   & TX2   & RX2   & 37.2  & 70.8 &     9.1  & NA \\
% \hline
%     LOS   & TX2   & RX6   & 97    & 72.2 &    58   & 76.8 \\
% \hline
%     LOS   & TX3   & RX5   & 19.3  & 64.8 &     20.8  & NA \\
% \hline
%     LOS   & TX4   & RX1   & 11.4  & 59.0 &    NA   & 77.8 \\
% \hline
%     NLOS  & TX1   & RX2   & 27    & 88.6 & 77.4 & 74.8 \\
% \hline
%     NLOS  & TX1   & RX3   & 37.6  & 89.9  & 62.6 & 55.9 \\
% \hline
%     NLOS  & TX2   & RX3   & 67.3  & 103   & 45 & 49.7 \\
% \hline
%    NLOS & TX2 & RX4 & 32.2 & 98.3 & 50.5 & 69.8 \\
% \hline
%     NLOS & TX2 & RX5 & 49 & 111.2 & 67 & 52.6 \\
% \hline
%     NLOS  & TX3   & RX1   & 12.3  & 72.6 & 27.7 & 50.2 \\
% \hline
%     NLOS  & TX3   & RX2   & 22.3  & 94.9 & 62.1 & 62.1 \\
% \hline
%     NLOS  & TX3   & RX3   & 65.6  & 88.9 & 32.8 & 68 \\
% \hline
%     NLOS  & TX3   & RX4   & 30    & 90 & 37.4 & 50.7 \\
% \hline
%     NLOS & TX3 & RX6 & 49.5 & 104.9 & 18.9 & NA \\
% \hline
%     NLOS  & TX4   & RX2   & 17.1  & 67.9 & 41.9 & 57.9 \\
% \hline
%     NLOS  & TX4   & RX3   & 87    & 94.2 & 23.4 & 73 \\
% \hline
%     NLOS  & TX4   & RX4   & 23.5  & 73.2 & 88.3 & 84.5 \\
%     \hline
%     \end{tabular}%
%   \label{tab:addlabel}%
% \end{table}%


% Table generated by Excel2LaTeX from sheet 'Sheet1'
% \begin{table}[htbp]
%   \centering
%   \caption{Add caption}
%     \begin{tabular}{|c|p{1.6em}|p{1.6em}|p{1.8em}|p{2.4em}|p{1.9em}|p{2em}|}
%     \hline
%     \multicolumn{7}{|c|}{16.95 GHz Omnidirectional V-V PL, DS and ASA} \\
%     \hline
%     Env.  & TX ID & RX ID & T-R (m) & PL (dB) & DS (ns) & ASA ($^\circ$) \\
%     \hline
%     LOS   & TX1   & RX1   & 24.6  & 73.8  & 15.6 & 6.7 \\
%     \hline
%     LOS   & TX1   & RX4   & 51    & 83.8 & 10  & 3.1 \\
%     \hline
%     LOS   & TX2   & RX1   & 64    & 82.6 & 21.3 & 71.6 \\
%     \hline
%     LOS   & TX2   & RX2   & 37.2  & 79.3  & 27.3 & NA \\
%     \hline
%     LOS   & TX2   & RX6   & 97    & 80.3  & 60.2 & NA \\
%     \hline
%     LOS   & TX3   & RX5   & 19.3  & 73.2 & 9.1  & NA \\
%     \hline
%     LOS   & TX4   & RX1   & 11.4  & 67.2 & 11.4 & 56.1 \\
%     \hline
%     NLOS  & TX1   & RX2   & 27    & 98.9 & 40.4 & 64.7 \\
%     \hline
%     NLOS  & TX1   & RX3   & 37.6  & 100.9 & 51.3 & 45.3 \\
%     \hline
%     NLOS  & TX2   & RX3   & 67.3  & 109.8 & 46.6 & 15.2 \\
%     \hline
%     NLOS & TX2 & RX4 & 32.2 & 107.9 & 45 & 46.4 \\
%     \hline
%     NLOS & TX2 & RX5 & 49 & 124.4 & 16.5 & 13.9 \\
%     \hline
%     NLOS  & TX3   & RX1   & 12.3  & 87.3 & 23.8 & 68 \\
%     \hline
%     NLOS  & TX3   & RX2   & 22.3  & 111.3 & 65.7 & 6.2 \\
%     \hline
%     NLOS  & TX3   & RX3   & 65.6  & 100.6 & 31.3 & 72.3 \\
%     \hline
%     NLOS  & TX3   & RX4   & 30    & 96.8 & 51.6 & 54.6 \\
%     \hline
%    NLOS & TX3 & RX6 & 49.5 & 119.7 & 17.7 & 4.8 \\
%     \hline
%     NLOS  & TX4   & RX2   & 17.1  & 93.3 & 52 & 83.8 \\
%     \hline
%     NLOS  & TX4   & RX3   & 87    & 110.7 & 9.4  & 6.7 \\
%     \hline
%     NLOS  & TX4   & RX4   & 23.5  & 91.9 & 76.9 & 81.7 \\
%     \hline
%     \end{tabular}%
%   \label{tab:addlabel}%
% \end{table}%
